# Supplementary material for: BpForms and BcForms: Tools for concretely describing non-canonical polymers and complexes to facilitate comprehensive biochemical networks
Source: arXiv:1903.10042 ancillary file (2019-09-03)
Supplement: Supplementary file 1 [file Additional-File-1.pdf]

# *BpForms* and *BcForms*: Additional File 1, Figure S1, and Tables S1-S5

Paul F. Lang[1,2,3,*], Yassmine Chebaro[1,2,4,*], Xiaoyue Zheng[1,2,*], John A. P. Sekar[1,2], Bilal Shaikh[1,2], Darren A. Natale[5], and Jonathan R. Karr[1,2,**]

[1]Icahn Institute, Icahn School of Medicine at Mount Sinai, US
[2]Department of Genetics & Genomic Sciences, Icahn School of Medicine at Mount Sinai, US
[3]Department of Biochemistry, Oxford University, UK
[4]Institut de Génétique et de Biologie Moléculaire et Cellulaire, FR
[5]Protein Information Resource, Georgetown University Medical Center, US

[*]These authors contributed equally to this work
[**]Correspondence: karr@mssm.edu

## Contents

**1 Features of the *BpForms-BcForms* toolkit** **2**

**2 Overview of the grammars for polymers and complexes** **2**
- 2.1 *BpForms* grammar for polymers . . . 2
- 2.2 *BcForms* grammar for complexes . . . 4

**3 Formal descriptions of the grammars for polymers and complexes** **4**
- 3.1 *BpForms* grammar for polymers . . . 5
- 3.2 *BcForms* grammar for complexes . . . 7

**4 Coordinate system** **8**

**5 Construction of the alphabets of DNA, RNA, and protein residues** **9**

**6 Construction of the ontology of crosslinks** **9**

**7 Semantic verification of polymers and complexes** **9**

**8 Visualizations of polymers and complexes** **10**

**9 Integration with omics and systems and synthetic biology formats** **10**
- 9.1 FASTA format for DNA, RNA, and protein sequences . . . 10
- 9.2 BioPAX format for pathways . . . 10
- 9.3 CellML and SBML formats for kinetic models . . . 11
- 9.4 Synthetic Biology Open Language (SBOL) format for genetic designs . . . 11

**10 Implementation** **12**

**11 Comparison with other formats and alphabet-like resources** **12**
- 11.1 Comparison of *BpForms* grammar with other formats for polymers . . . 12
- 11.2 Comparison of *BpForms* alphabets with other alphabet-like resources . . . 16
- 11.3 Comparison of the *BpForms* crosslink ontology with other resources . . . 17
- 11.4 Comparison of *BcForms* grammar with other formats for complexes . . . 17

**12 Case studies** **18**

**13 Acronyms** **18**

# 1. Features of the *BpForms-BcForms* toolkit

The toolkit has the following features:

- **Concrete:** To help researchers communicate and integrate data about macromolecules, the grammars can capture the primary structures of macromolecules, including non-canonical residues, caps, crosslinks, and nicks.
- **Abstract:** To facilitate network-scale research, *BpForms* and *BcForms* use alphabets of residues and an ontology of crosslinks to abstract the structures of polymers and complexes.
- **Extensible:** To capture any polymer or complex, users can define residues and complexes inline or define custom alphabets and ontologies.
- **Structured coordinates:** To compose residues and crosslinks into polymers and complexes, each subunit, residue, and atom has a unique coordinate relative to its parent.
- **Context-free:** To help integrate information about the processes which synthesize and modify macromolecules, the grammars capture the structures of macromolecules separately from the processes which generate macromolecules.
- **User-friendly:** To ensure *BpForms* and *BcForms* is easy to use, the grammars are human-readable, and the toolkit includes web applications and command-line programs.
- **Machine-readable:** The grammars are machine-readable to enable analyses of macromolecules.
- **Composable:** To facilitate network-scale research, we have developed protocols for composing the grammars with formats such as BioPAX, CellML, SBML, and SBOL.
- **Backward-compatible:** *BpForms* is backward compatible with the IUPAC/IUBMB format to maximize compatibility with existing formats, software, and knowledge.

# 2. Overview of the grammars for polymers and complexes

## 2.1. *BpForms* grammar for polymers

*BpForms* describes polymers using a similar grammar to the IUPAC/IUBMB format. For example, `GaTC` describes a DNA 4-mer which contains 6-methyladenine (a) at the second residue. `RCAC | x-link: [type: "disulfide" | l: 2 | r: 4]` describes a protein 4-mer which contains a disulfide bond between the cysteines at the second and fourth positions. `AUUCG | circular` describes a circular RNA 5-mer.

Here, we summarize the grammar. Box 1 and https://bpforms.org contain several examples of polymers encoded in the grammar. Section 3.1 contains a formal description of the grammar.

### Residue sequence

Residues that belong to alphabets can be indicated by their codes. Residues which have single-character codes can be indicated by their codes. For example, `A` describes deoxyadenosine monophosphate. Residues which have multiple-character codes can be indicated by enclosing their codes in brackets. For example, `{m2C}` describes 2-O-methylcytidine monophosphate.

Residues which are not in the alphabets can be described in three ways: users can submit pull requests to add residues to the public alphabets, define their own alphabets, or define residues inline within descriptions of polymers.

*User-defined residues.* Residues can be defined inline as a pipe-separated set of attribute-value pairs enclosed in brackets. For example, `[name: "m6G" | ...]` describes 6-O-methylguanosine monophosphate ($m^2G$). The `structure` attribute can capture the molecular structure of the residue in the SMILES format. For example, `structure: "COc1nc(N)nc2c1ncn2C1CC(C(O1)COP(=O)([-])[O-])O"` represents the structure of $m^2G$. Optionally, the `l-bond-atom` and `r-bond-atom` attributes can capture the atoms which can form bonds with preceding (l, left) and following (r, right) residues, and the `l-displaced-atom` and `r-displaced-atom` attributes can capture the atoms which are displaced by the formation of these bonds. The values of these attributes indicate the element, coordinate, and change in the formal charge of each atom upon bonding an adjacent residue. For example, `l-bond-atom: P20` indicates the phosphorous of $m^6G$ that forms bonds with preceding residues and `l-displaced-atom: O23-1` indicates the oxygen which is displaced by the formation of these bonds.

Several optional attributes can capture metadata about residues. The `id`, `name`, and `synonym` attributes can capture labels. The `identifier` attribute can capture references to equivalent entries in databases. For example, `identifier: "6-O-methylguanine" @ "dnamod"` indicates a reference to an entry in DNAmod. The `base-monomer` attribute can indicate how residues are synthesized from other residues. For example, `base-monomer: "G"` indicates that $m^6G$ is derived from guanosine (G). The `comments` attribute can capture additional information about residues.

## Crosslinks

*BpForms* represents each crosslink between two residues as (a) a pair of the atoms which form a bond between the residues and (b) a set of the atoms which are displaced by the formation of the bond. Crosslinks which belong to the ontology of crosslinks can be described by the `x-link` keyword followed by a pipe-separated list of attribute-value pairs enclosed in brackets. The `type` attribute indicates the type of the crosslink. The value of this attribute must refer to an entry in the crosslinks ontology. The `l` and `r` attributes indicate the coordinates of the residues involved in the crosslink. For example, `x-link: [type: "disulfide" | l: 2 | r: 5]` indicates a disulfide bond between cysteines at the second and fifth residues.

Users can also define crosslinks by submitting pull requests to add crosslinks to the public ontology, defining their own ontology, or defining crosslinks inline within descriptions of polymers.

*User-defined crosslinks.* Crosslinks can be defined inline as a pipe-separated set of attribute-value pairs enclosed in brackets. Similar to user-defined residues, the `l-bond-atom` and `r-bond-atom` attributes describe the atoms which form covalent bonds and the `l-displaced-atom` and `r-displaced-atom` attributes describe the atoms which are displaced by the formation of these bonds. For example, `l-bond-atom: 2O11-1 | r-bond-atom: 7P20` indicates that the crosslink involves a covalent bond between the oxygen at the eleventh position of the second residue and the phosphorous at the twentieth position of the seventh residue, and that the formation of the crosslink decreases the formal charge of the oxygen by one electron. The `order` attribute can capture the order (single, double, triple, or aromatic) of the bond. The `stereo` attribute can capture the stereochemistry (wedge, hash, up, or down) of the bond. The `comments` attribute can capture additional textual information about the crosslink.

## Nicks

Nicks can be defined by inserting a colon between the residues involved in the nick. For example, `AC:DE` describes a nick between the second and third residues of a peptide.

### Linear or circular topology

Optionally, the `circular` attribute can describe a bond between the left bonding site of the first residue and the right bonding site of the last residue. For example, `CTAC | circular` describes a circular DNA tetramer.

### Missing knowledge

User-defined residues can also capture four types of uncertainty about polymers. The `delta-mass` and `delta-charge` attributes can describe mass and charge which have been observed, but which cannot be assigned to an exact molecular structure. For example, `[id: "R" | delta-mass: 17 | delta-charge: 0]` indicates a residue whose mass is 17 Da greater than that of arginine, but whose exact structure is not known. The `position` attribute can capture uncertainty about the location and biosynthesis of a non-canonical residue. For example, `AC[base-monomer: "Y" | identifier: "MOD:00696" @ "mod" | position: 3-5 [S, T, Y]]ST` indicates a peptide that contains a phosphorylated serine, threonine, or tyrosine between positions five and ten.

## 2.2. *BcForms* grammar for complexes

*BcForms* describes complexes using a grammar that is similar to a linear mathematical expression. For example, `CHAF1A + SUMO1 | x-link: [ ...]` describes a crosslinked heterodimer of chromatin assembly factor 1 subunit A (CHAF1A) and small ubiquitin-related modifier 1 (SUMO1).

Here, we summarize the grammar. Box 2 and https://bcforms.org contain examples of complexes encoded in the grammar. Section 3.2 contains a formal description of the grammar.

### Subunit composition

The subunits involved in complexes and their stoichiometries can be described as a linear expression. For example, `2 * HBA1 + 2 * HBB` describes hemoglobin HbA, a heterotetramer composed of two subunits of HBA1 (UniProt: P69905) and two subunits of HBB (UniProt: P68871). Each subunit can be represented using *BpForms* or SMILES.

### Intersubunit crosslinks

*BcForms* captures crosslinks similar to *BpForms*. Crosslinks which belong to the ontology can be described using the coordinates of the residues involved in the crosslink. For example, `x-link: [type: "disulfide" | l: P83658(1)-7 | r: P83658(2)-12 | ...]` describes a disulfide bond between the seventh and twelfth cysteines of two subunits of disintegrin schistatin (UniProt: P83658). The `l` and `r` attributes describe the subunit type, subunit coordinate, and residue coordinate of the atoms involved in the crosslink. Users can also define crosslinks inline similarly to *BpForms*. For example, `x-link: [l-bond-atom: P83658(1)-7S11 | r-bond-atom: P83658(2)-12S11 | ...]` describes the same disulfide bond between the seventh and twelfth cysteines of disintegrin schistatin.

Complexes can have zero, one, or more crosslinks. Each crosslink can involve the formation of one or more covalent bonds and the displacement of zero or more atoms.

# 3. Formal descriptions of the grammars for polymers and complexes

The *BpForms* and *BcForms* grammars are defined in Extended Backus-Naur Form (EBNF) [1] using Lark [2]. The grammars are available at https://github.com/KarrLab. Below are descriptions of the grammars in Backus-Naur Form (BNF).

## 3.1. *BpForms* grammar for polymers

*BpForm*

⟨bpform⟩ ⊨ ⟨seq⟩ ⟨x-links⟩ ⟨circularity⟩

*Sequence of residues and nicks*

⟨seq⟩ ⊨ ⟨residue⟩ | ⟨residue⟩ ⟨seq⟩ | *nick* ⟨residue⟩ ⟨seq⟩

⟨residue⟩ ⊨ ⟨single-code-residue⟩ | ⟨delimited-multi-code-residue⟩ | ⟨user-residue⟩

*Alphabet-defined residues*

⟨single-code-residue⟩ ⊨ ⟨code⟩

⟨delimited-multi-code-residue⟩ ⊨ `{` ⟨multi-code⟩ `}`

⟨code⟩ ⊨ *non-whitespace character*

⟨multi-code⟩ ⊨ ⟨code⟩ | ⟨code⟩ ⟨multi-code⟩

*User-defined residues*

⟨user-residue⟩ ⊨ `[` ⟨attrs⟩ `]`

⟨attrs⟩ ⊨ ⟨attr⟩ | ⟨attr⟩ `'|'` ⟨attrs⟩ | $\lambda$

⟨attr⟩ ⊨ ⟨id⟩ | ⟨name⟩ | ⟨synonym⟩ | ⟨identifier⟩ | ⟨structure⟩ | ⟨atom⟩ | ⟨base⟩ | ⟨delta-mass⟩ | ⟨delta-charge⟩ | ⟨position⟩ | ⟨comments⟩

⟨id⟩ ⊨ `id :` `"` ⟨escaped-string⟩ `"`

⟨name⟩ ⊨ `name :` `"` ⟨escaped-string⟩ `"`

⟨synonym⟩ ⊨ `synonym :` `"` ⟨escaped-string⟩ `"`

⟨identifier⟩ ⊨ `identifier :` `"` ⟨identifier-ns⟩ `" @ "` ⟨identifier-id⟩ `"`

⟨identifier-ns⟩ ⊨ ⟨escaped-string⟩

⟨identifier-id⟩ ⊨ ⟨escaped-string⟩

⟨structure⟩ ⊨ `structure :` `"` ⟨string⟩ `"`

⟨atom⟩ ⊨ ⟨atom-type⟩ `:` ⟨atom-element⟩ ⟨atom-index⟩ ⟨atom-charge⟩

⟨base⟩ ⊨ `base-monomer :` `"` ⟨multi-code⟩ `"`

⟨delta-mass⟩ ⊨ `delta-mass :` ⟨number⟩

⟨delta-charge⟩ ⊨ `delta-charge :` ⟨integer⟩

⟨position⟩ ⊨ `position :` ⟨position-start⟩ `-` ⟨position-end⟩ ⟨position-residues⟩

⟨position-start⟩ ⊨ ⟨positive-integer⟩

⟨position-end⟩ ⊨ ⟨positive-integer⟩

⟨position-residues⟩ ⊨ `[` ⟨position-residue-codes⟩ `]` | $\lambda$

⟨position-residue-codes⟩ ⊨ ⟨multi-code⟩ | ⟨multi-code⟩ `'|'` ⟨position-residue-codes⟩

⟨comments⟩ ⊨ `comments :` `"` ⟨escaped-string⟩ `"`

| | | |
|---|---|---|
| *Crosslinks* | | |
| ⟨x-links⟩ | $\models$ | ⟨x-link⟩ \| ⟨x-link⟩ ⟨x-links⟩ \| $\lambda$ |
| ⟨x-link⟩ | $\models$ | `'|'` `x-link` `:` `[` ⟨x-link-attrs⟩ `]` |
| ⟨x-link-attrs⟩ | $\models$ | ⟨onto-x-link-attrs⟩ \| ⟨user-x-link-attrs⟩ |
| ⟨onto-x-link-attrs⟩ | $\models$ | ⟨onto-x-link-attr⟩ \| ⟨onto-x-link-attr⟩ `'|'` ⟨onto-x-link-attrs⟩ |
| ⟨onto-x-link-attr⟩ | $\models$ | ⟨onto-x-link-type⟩ \| ⟨onto-x-link-l-monomer⟩ \| ⟨onto-x-link-r-monomer⟩ |
| ⟨onto-x-link-type⟩ | $\models$ | `type` `:` `"` ⟨non-whitespace-characters⟩ `"` |
| ⟨onto-x-link-l-monomer⟩ | $\models$ | `l` `:` ⟨positive-integer⟩ |
| ⟨onto-x-link-r-monomer⟩ | $\models$ | `r` `:` ⟨positive-integer⟩ |
| *User-defined crosslinks* | | |
| ⟨user-x-link-attrs⟩ | $\models$ | ⟨user-x-link-attr⟩ \| ⟨user-x-link-attr⟩ `'|'` ⟨user-x-link-attrs⟩ \| $\lambda$ |
| ⟨user-x-link-attr⟩ | $\models$ | ⟨user-x-link-atom⟩ \| ⟨user-x-link-order-attr⟩ \| ⟨user-x-link-stereo-attr⟩ \| ⟨user-x-link-comments-attr⟩ |
| ⟨user-x-link-atom⟩ | $\models$ | ⟨atom-type⟩ ⟨atom-residue⟩ ⟨atom-element⟩ ⟨atom-index⟩ ⟨atom-charge⟩ |
| ⟨user-x-link-order-attr⟩ | $\models$ | `order` `:` `"`⟨user-x-link-order⟩ `"` |
| ⟨user-x-link-order⟩ | $\models$ | `single` \| `double` \| `triple` \| `aromatic` |
| ⟨user-x-link-stereo-attr⟩ | $\models$ | `stereo` `:` `"`⟨user-x-link-stereo⟩ `"` |
| ⟨user-x-link-stereo⟩ | $\models$ | `wedge` \| `hash` \| `up` \| `down` |
| ⟨user-x-link-comments-attr⟩ | $\models$ | `commments` `:` `"` ⟨escaped-string⟩ `"` |
| *nicks* | | |
| ⟨nick⟩ | $\models$ | `:` |
| *Circularity* | | |
| ⟨circularity⟩ | $\models$ | `'|'` `circular` \| $\lambda$ |
| *User-defined atoms* | | |
| ⟨atom-type⟩ | $\models$ | `l-bond-atom` \| `l-displaced-atom` \| `r-bond-atom` \| `r-displaced-atom` |
| ⟨atom-residue⟩ | $\models$ | ⟨positive-integer⟩ |
| ⟨atom-element⟩ | $\models$ | `A...Z` \| `A...Z a...z` |
| ⟨atom-index⟩ | $\models$ | ⟨positive-integer⟩ |
| ⟨atom-charge⟩ | $\models$ | ⟨sign⟩ ⟨non-negative-integer⟩ \| $\lambda$ |
| ⟨sign⟩ | $\models$ | `+` \| `-` |
| *Primitives* | | |

⟨string⟩ ⊨ *string*

⟨escaped-string⟩ ⊨ *quote escaped string*

⟨non-whitespace-characters⟩ ⊨ *non-whitespace characters*

⟨integer⟩ ⊨ *integer*

⟨positive-integer⟩ ⊨ *positive integer*

⟨non-negative-integer⟩ ⊨ *non-negative integer*

## 3.2. *BcForms* grammar for complexes

*BcForm*

⟨bcform⟩ ⊨ ⟨subunits⟩ ⟨x-links⟩

*Subunits*

⟨subunits⟩ ⊨ ⟨subunit⟩ | ⟨subunit⟩ + ⟨subunits⟩

⟨subunit⟩ ⊨ ⟨coefficient⟩ * ⟨id⟩ | ⟨id⟩

⟨id⟩ ⊨ ⟨non-white space characters⟩

⟨coefficient⟩ ⊨ ⟨positive integer⟩

*Crosslinks*

⟨x-links⟩ ⊨ ⟨x-link⟩ | ⟨x-link⟩ ⟨x-links⟩

⟨x-link⟩ ⊨ `‘|’ crosslink : [` ⟨x-link-attrs⟩ `]`

⟨x-link-attrs⟩ ⊨ ⟨onto-x-link-attrs⟩ | ⟨user-x-link-attrs⟩

⟨onto-x-link-attrs⟩ ⊨ ⟨onto-x-link-attr⟩ | ⟨onto-x-link-attr⟩ `‘|’` ⟨onto-x-link-attrs⟩

⟨onto-x-link-attr⟩ ⊨ ⟨onto-x-link-type⟩ | ⟨onto-x-link-l-monomer⟩ | ⟨onto-x-link-r-monomer⟩

⟨onto-x-link-type⟩ ⊨ `type : "` ⟨onto-x-link-type-value⟩ `"`

⟨onto-x-link-type-value⟩ ⊨ ⟨non-whitespace characters⟩

⟨onto-x-link-l-monomer⟩ ⊨ `l :` ⟨atom-subunit-id⟩ `(` ⟨atom-subunit-index⟩ `) -` ⟨atom-monomer-index⟩

⟨onto-x-link-r-monomer⟩ ⊨ `r :` ⟨atom-subunit-id⟩ `(` ⟨atom-subunit-index⟩ `) -` ⟨atom-monomer-index⟩

*User-defined crosslinks*

⟨user-x-link-attrs⟩ ⊨ ⟨user-x-link-attr⟩ | ⟨user-x-link-attr⟩ `‘|’` ⟨user-x-link-attrs⟩

⟨user-x-link-attr⟩ ⊨ ⟨user-x-link-atom⟩ | | ⟨user-x-link-order-attr⟩ | ⟨user-x-link-stereo-attr⟩ | ⟨user-x-link-comments-attr⟩

⟨user-x-link-order-attr⟩ ⊨ `order : "`⟨user-x-link-order⟩ `"`

⟨user-x-link-order⟩ ⊨ `single | double | triple | aromatic`

| | | |
|---|---|---|
| ⟨user-x-link-stereo-attr⟩ | ⊨ | `stereo : "`⟨user-x-link-stereo⟩ `"` |
| ⟨user-x-link-stereo⟩ | ⊨ | `wedge` \| `hash` \| `up` \| `down` |
| ⟨user-x-link-comments-attr⟩ | ⊨ | `commments : "` ⟨escaped-string⟩ `"` |
| *User-defined atoms* | | |
| ⟨user-x-link-atom⟩ | ⊨ | ⟨atom-type⟩ `:` ⟨atom-subunit-id⟩ `(` ⟨atom-subunit-index⟩ `)` `-` ⟨atom-monomer-index⟩ ⟨atom-index⟩ ⟨atom-element⟩ ⟨atom-charge⟩ |
| ⟨atom-type⟩ | ⊨ | `l-bond-atom` \| `r-bond-atom` \| `l-displaced-atom` \| `r-displaced-atom` |
| ⟨atom-subunit-id⟩ | ⊨ | ⟨non-whitespace characters⟩ |
| ⟨atom-subunit-index⟩ | ⊨ | ⟨positive integer⟩ |
| ⟨atom-monomer-index⟩ | ⊨ | ⟨positive integer⟩ |
| ⟨atom-index⟩ | ⊨ | ⟨positive integer⟩ |
| ⟨atom-element⟩ | ⊨ | `A...Z` \| `A...Z a...z` |
| ⟨atom-charge⟩ | ⊨ | ⟨sign⟩ ⟨atom-charge-value⟩ \| $\lambda$ |
| ⟨sign⟩ | ⊨ | `+` \| `-` |
| ⟨atom-charge-value⟩ | ⊨ | ⟨non-negative integer⟩ |
| *Primitives* | | |
| ⟨escaped-string⟩ | ⊨ | *quote escaped string* |
| ⟨non-whitespace-characters⟩ | ⊨ | *non-whitespace characters* |
| ⟨positive-integer⟩ | ⊨ | *positive integer* |
| ⟨non-negative-integer⟩ | ⊨ | *non-negative integer* |

## 4. Coordinate system

To facilitate descriptions of crosslinks, each residue, and atom represented by *BpForms* has a unique coordinate (Figure 2). The coordinate of each residue is its position within the residue sequence of its parent polymer. The coordinate of each atom is a tuple of the coordinate of its parent residue and its position within the canonical SMILES ordering of the atoms in its parent residue prior to incorporation into polymers.

Each subunit, residue, and atom represented by *BcForms* also has a unique coordinate (Figure 2). The coordinates of repeated subunits range from one to the stoichiometry of the subunit. The coordinate of each residue is a two-tuple of the coordinate of its parent subunit and its position within the residue sequence of its parent subunit. The coordinate of each atom is a three-tuple of the coordinate of its parent subunit, the position of its parent residue within the residue sequence of its parent polymer, and its position within the canonical SMILES ordering of its parent residue.

# 5. Construction of the alphabets of DNA, RNA, and protein residues

To support a broad range of research, we developed the alphabets of DNA, RNA, and protein residues by merging residues from multiple databases. We developed the DNA alphabet by combining the deoxyribose nucleotide monophosphates and 3' and 5' DNA caps from the PDB Chemical Component Dictionary (PDB CCD) [3] with the verified DNA nucleobases from DNAmod [4] and the deoxyribose nucleosides from REPAIRtoire [5] that had concrete structures. We developed the RNA alphabet by combining the ribose nucleotide monophosphates and 3' and 5' RNA caps from the PDB CCD with the ribose nucleosides from MODOMICS [6] and the RNA Modification Database [7] that had concrete structures. We developed the protein alphabet by merging residues from the PDB CCD and RESID [8].

First, we downloaded, scraped, and manually extracted residues from DNAmod, MODOICS, PDB CCD, REPAIRtoire, RESID, the RNA Modification Database. Second, we parsed each database into a list of residues. Third, we rejected residues with incompletely defined structures, as well as inconsistent residues such as nucleotides from DNAmod. Fourth, we normalized the DNA and RNA residues to nucleotide monophosphates and normalized the protein residues to amino acids. For example, we transformed the DNAmod entries to nucleotides by adding deoxyribose monophosphate to each nucleobase. Fifth, we merged the repeated residues. This included residues that had the same molecular structure, that the upstream sources annotated were equivalent, or that had similar names. Lastly, we identified the indices of the forward and reverse bonding sites in each residue. This included the 3' and 5' atoms in each DNA and RNA residue and the carboxyl and amino atoms in each protein residue.

We automated the alphabet construction process by writing scripts to build each alphabet. Going forward, this will enable us to periodically incorporate updates to the upstream databases into the alphabets.

# 6. Construction of the ontology of crosslinks

We developed the ontology of crosslinks based on entries in RESID which represent crosslinked dimers. First, we searched RESID for entries which represent crosslinked dimers. Second, we identified the individual residues which participate in each dimer. Third, we used ChemAxon Marvin [9] to identify the atoms involved in each crosslink. Next, we used Open Babel [10] to determine the indices of these atoms. Finally, we manually assigned an id and name to each crosslink.

# 7. Semantic verification of polymers and complexes

To help quality control information about macromolecules, *BpForms* and *BcForms* have methods for verifying the semantic correctness of polymers and complexes. The *BpForms* verification method checks that each residue has a defined structure, each atom that bonds an adjacent residue has a defined element and position which is consistent with the structure of its parent residue, and each pair of consecutive residues can form a bond. The method also checks that the element and position of each atom in each crosslink are consistent with the structure of its parent residue.

The *BcForms* verification method checks that each subunit is semantically concrete and the element and position of each atom in each crosslink are consistent with the structure of its parent residue. For example, these methods can identify invalid proteins that contain consecutive residues which cannot bond because the first residue lacks a carboxyl terminus or the second residue lacks an amino terminus.

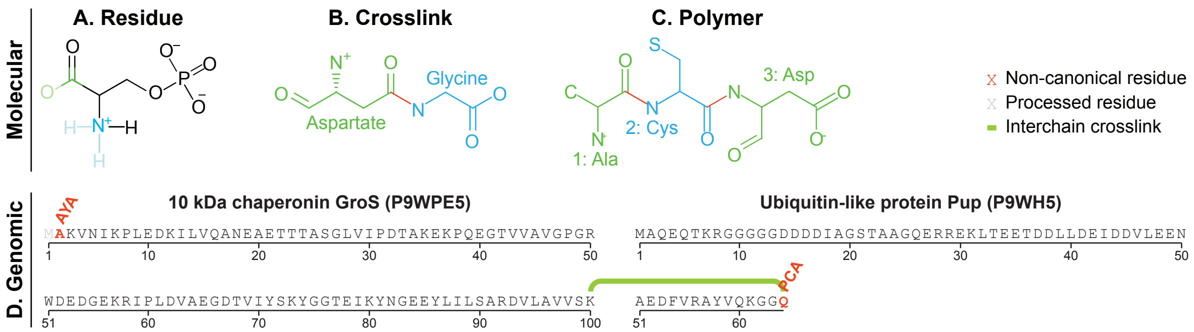


**Figure S1. Molecular and genomic visualizations of polymers and complexes that can be generated with *BpForms* and *BcForms*.** *BpForms* can generate molecular visualizations of residues such as phosphoserine (**A**), crosslinks such as an isoaspartyl glycine isopeptide bond (**B**), and polymers such as the tripeptide ACD (**C**). The blue and green letters in (A) indicate the atoms which can bond with preceding and following residues; the light blue and light green letters indicate the atoms which are displaced by the formation of these bonds. The blue and green elements in (B) indicate the individual residues involved in the crosslink; the red line indicates the covalent bond that crosslinks the residues. The green elements in (C) indicate the first and third residues in the peptide, the blue elements indicate the second residue, and the red lines indicate the covalent bonds between the residues. *BpForms* and *BcForms* can also generate sequence-based visualizations of polymers and complexes such as the pupylation of chaperonin GroS (**D**, UniProt: P9WPE5, P9WH5). The gray letter indicates a residue which is removed post-translationally, the red letters indicate the residues which are post-translationally modified, and the green line indicates the residues which are post-translationally crosslinked.

# 8. Visualizations of polymers and complexes

*BpForms* and *BcForms* can generate several molecular and genomic visualizations of residues, crosslinks, polymers, and complexes. Figure S1 contains examples of these visualizations.

# 9. Integration with omics and systems and synthetic biology formats

## 9.1. FASTA format for DNA, RNA, and protein sequences

Box S1 illustrates how *BpForms* can be integrated with the FASTA format [11] to describe multiple non-canonical DNA, RNA, or proteins within a single file. The *BpForms* Python library includes methods for importing and exporting *BpForms* to and from FASTA documents. *BpForms*-encoded FASTA documents can also be read and written by standard FASTA tools such as Biopython [12].

## 9.2. BioPAX format for pathways

BioPAX [13] is a format for describing biochemical pathways such as metabolism. Box S2 illustrates how *BpForms* can be integrated with BioPAX to describe the polymers that participate in pathways. Users who need to describe residues and crosslinks which are not part of the public *BpForms* ontologies can either describe the residues and crosslinks inline inside descriptions of polymers, build custom alphabets of residues and a custom ontology of crosslinks and bundle these documents with BioPAX documents into COMBINE archives [14], or submit Git pull requests to add residues and crosslinks to the public alphabets and ontology. By helping BioPAX describe the polymers involved in pathways, *BpForms* can make pathways easier to understand and combine into comprehensive maps of cells. Unfortunately, there is no straightforward way to integrate *BcForms* with BioPAX because BioPAX's data model for complexes is not extensible.

## 9.3. CellML and SBML formats for kinetic models

CellML [15] and the Systems Biology Markup Language (SBML) [16] are formats for describing kinetic models. Both formats have limited capabilities to describe the semantic meaning of model elements which represent macromolecules because both formats encourage users to annotate the meaning of model elements by referencing entities in databases such as UniProt [17] which do not represent every possible form of every macromolecule. For example, CellML and SBML cannot capture the differences among the monophosphorylated states of MAPK because UniProt does not have distinct entries for each state.

Boxes S3 and S4 illustrate how *BpForms* and *BcForms* can be integrated with CellML and SBML to describe the macromolecules represented by models. Users who need to describe residues and crosslinks which are not part of the public *BpForms* ontologies can either describe the residues and crosslinks inline inside descriptions of polymers, build custom alphabets of residues and a custom ontology of crosslinks and bundle these documents with CellML and SBML documents into COMBINE archives [14], or submit Git pull requests to add residues and crosslinks to the public ontologies.

By describing the semantic meaning of model elements, *BpForms* and *BcForms* can make models easier to understand, compare, extend, and combine into more comprehensive models such as whole-cell (WC) models [18, 19].

## 9.4. Synthetic Biology Open Language (SBOL) format for genetic designs

SBOL [22] is a format for describing genetic designs for synthetic organisms. Box S5 illustrates how *BpForms* can be integrated with SBOL to concretely describe the DNA, RNA, and protein parts of genetic designs. Users who need to describe residues and crosslinks which are not part of the public *BpForms* ontologies can either describe the residues and crosslinks inline inside descriptions of polymers, build custom alphabets of residues and a custom ontology of crosslinks and bundle these documents with SBOL documents into COMBINE archives [14], or submit Git pull requests to add residues and crosslinks to the public alphabets and ontology. In SBOL PEP 033 [23], we formally proposed this integration between *BpForms* and SBOL to the SBOL community. Unfortunately, there is no straightforward way to integrate *BcForms* with SBOL because SBOL's data model for complexes is not extensible. Instead, we encourage the SBOL community to expand SBOL to capture stoichiometric, crosslink, and nick information about complexes.

By helping capture the structures of parts, *BpForms* can help bioengineers identify the biosynthetic dependencies of parts and, in turn, identify constraints on the transformation of parts into new hosts. For example, *BpForms* can help bioengineers identify post-translational modification enzymes that must be co-transformed with parts to synthesize modifications that are essential to the parts.

```
> yp | phosphorylated MEK | Q02750 | pS218
MPKKKPTPIQLNPAPDGSAVNGTSSAETNLEALQKKLEELELDEQQRKRLEAFLTQKQKVGELKDDDFEKISELGAGNGGVVFKV
SHKPSGLVMARKLIHLEIKPAIRNQIIRELQVLHECNSPYIVGFYGAFYSDGEISICMEHMDGGSLDQVLKKAGRIPEQILGKVS
IAVIKGLTYLREKHKIMHRDVKPSNILVNSRGEIKLCDFGVSGQLID{AA0037}MANSFVGTRSYMSPERLQGTHYSVQSDIWS
MGLSLVEMAVGRYPIPPPDAKELELMFGCQVEGDAAETPPRPRTPGRPLSSYGMDSRPPMAIFELLDYIVNEPPPKLPSGVFSLE
FQDFVNKCLIKNPAERADLKQLMVHAFIKRSDAEEVDFAGWLCSTIGLNQPSTPTHAAGV
```

**Box S1.** ***BpForms* can be integrated with the FASTA format to describe multiple polymers within a single document.** For example, a FASTA document can contain a *BpForms*-encoded description of monophosphorylated MAPK (UniProt: Q02750).

```
...
<bp:DNA>
   <bp:entityReference>
      <bp:DNAReference>
         <bp:sequence
            rdf:datatype="http://www.w3.org/2001/XMLSchema#string"
            rdf:about="http://edamontology.org/format_3909#dna">
            ...
            TGATTTGCCGTGGCGAGAAAATGTCG{a}TCGCCATTATGGCCGGCGTATTAGAAGCGCGCGGTCAC
            AACGTTACTGTTATCG{a}TCCGGTCGAAAAACTGCTGGCAGTGGGGCATTACCTCGAATCTACCGT
            ...
         </bp:sequence>
      </bp:DNAReference>
   </bp:entityReference>
</bp:DNA>
...
```

**Box S2. *BpForms* can help BioPAX documents describe the polymers involved in pathways.** For example, *BpForms* can help BioPAX capture the DNA methylation (orange) that helps *Escherichia coli* detect and degrade foreign DNA. Positions 701 to 800 of *E. coli*'s genome are shown.

# 10. Implementation

We implemented *BpForms* and *BcForms* with Python 3 [24] and several additional packages. We described the grammar in EBNF, and used Lark [2] to implement a parser for the grammar. We built the alphabets using BeautifulSoup [25], ChemAxon Marvin [9], Open Babel [10], Requests [26], and SQLAlchemy [27]. We described the alphabets in YAML Ain't Markup Language [28], and used ruamel.yaml [29] to parse the alphabets. We used Open Babel and Marvin to implement calculations of properties of macromolecules. We used Marvin to implement the molecular visualizations, and implemented the genomic visualizations using Scalable Vector Graphics (SVG) [30]. We used BioPython [12] to implement methods for importing and exporting *BpForms*-encoded polymers to and from FASTA documents. We implemented the command-line interfaces with Cement [31] and implemented the REST APIs with Flask-RESTPlus [32]. We implemented the web applications using Zurb Foundation [33] and FancyBox [34].

We deployed the web applications on a virtual private server using used Passenger [35].

We used the unittest module [36] to develop over 250 tests to verify *BpForms* and *BcForms*. We used Coverage.py [37] to check that our tests are comprehensive.

We used reStructuredText [38] and Sphinx [39] to generate documentation for *BpForms* and *BcForms*. We used Jupyter [40] to develop interactive tutorials for *BpForms* and *BcForms*.

# 11. Comparison with other formats and alphabet-like resources

## 11.1. Comparison of *BpForms* grammar with other formats for polymers

Several text formats, such as ProForma [41], have been developed to represent the structure of DNA, RNA, and proteins. In addition, several container formats, such as BioPAX, have limited abilities to represent the structure of DNA, RNA, and proteins.

As described below and summarized in Table S1, we believe that *BpForms* is a better format for omics, systems biology, and synthetic biology research because it abstracts the complete molecular structure of DNA, RNA, and proteins as collections of residues, crosslinks, and nicks; *BpForms* can

```xml
...

<species metaid="cdc2k" name="cdc2k-p">
   <annotation>
      <rdf:RDF
         xmlns:rdf="http://www.w3.org/1999/02/22-rdf-syntax-ns#">
         <rdf:Description rdf:about="#cdc2k">
            <bpforms:ProteinForm xmlns:bpforms="https://bpforms.org">
               MENYQKVEKIGEG{AA0038}{AA0039}GVVYKARHKLSGRIVAMKKIRLEDESEGVPSTAIREISLLKE
               VNDENNRSNCVRLLDILHAESKLYLVFEFLDMDLKKYMDRISETGATSLDPRLVQKFTYQLVNGVNFCHSR
               RIIHRDLKPQNLLIDKEGNLKLADFGLARSFGVPLRNY{AA0038}HEIVTLWYRAPEVLLGSRHYSTGVD
               IWSVGCIFAEMIRRSPLFPGDSEIDEIFKIFQVLGTPNEEVWPGVTLLQDYKSTFPRWKRMDLHKVVPNGE
               EDAIELLSAMLVYDPAHRISAKRALQQNYLRDFH
            </bpforms:ProteinForm>
         </rdf:Description>
      </rdf:RDF>
   </annotation>
</species>

<species metaid="YP" name="p-cyclin">
   <annotation>
      <rdf:RDF xmlns:rdf="http://www.w3.org/1999/02/22-rdf-syntax-ns#">
         <rdf:Description rdf:about="#YP">
            <bpforms:ProteinForm xmlns:bpforms="https://bpforms.org">
               MTTRRLTRQHLLANTLGNNDENHPSNHIARAK{AA0037}{AA0037}LH{AA0037}{AA0037}EN{AA
               0037}LVNGKKATVSSTNVPKKRHALDDV{AA0037}NFHNKEGVPLASKNTNVRHTTASVSTRRALEEKS
               IIPATDDEPA{AA0037}KKRRQPSVFNSSVPSLPQHLSTKSHSVSTHGVDAFHKDQATIPKKLKKDVDER
               VVSKDIPKLHRDSVESPESQDWDDLDAEDWADPLMVSEYVVDIFEYLNELEIETMPSPTYMDRQKELAWKM
               RGILTDWLIEVHSRFRLLPETLFLAVNIIDRFLSLRVCSLNKLQLVGIAALFIASKYEEVMCPSVQNFVYM
               ADGGYDEEEILQAERYILRVLEFNLAYPNPMNFLRRISKADFYDIQTRTVAKYLVEIGLLDHKLLPYPPSQ
               QCAAAMYLAREMLGRGPWNRNLVHYSGYEEYQLISVVKKMINYLQKPVQHEAFFKKYASKKFMKASLFVRD
               WIKKNSIPLGDDADEDYTFHKQKRIQHDMKDEEW
            </bpforms:ProteinForm>
         </rdf:Description>
      </rdf:RDF>
   </annotation>
</species>

<species metaid="pM" name="p-cyclin_cdc2-p">
   <annotation>
      <rdf:RDF xmlns:rdf="http://www.w3.org/1999/02/22-rdf-syntax-ns#">
         <rdf:Description rdf:about="#YP">
            <bcforms:BcForm xmlns:bcforms="https://bcforms.org">
               YP + cdc2k
            </bcforms:BcForm>
         </rdf:Description>
      </rdf:RDF>
   </annotation>
</species>

...
```

**Box S3. *BpForms* can help SBML describe the semantic meaning of the macromolecules represented by models.** For example, *BpForms* can help SBML describe that the cdc2k variable of the Tyson cell cycle model [20] represents a tri-phosphorylated form of cyclin dependent kinase 1 (UniProt: P04551).

```
...
<component cmeta:id="ypp" name="ypp">
   <rdf:RDF xmlns:rdf="http://www.w3.org/1999/02/22-rdf-syntax-ns#">
      <rdf:Description rdf:about="#ypp">
         <bpforms:ProteinForm xmlns:bpforms="https://bpforms.org">
            MPKKKPTPIQLNPAPDGSAVNGTSSAETNLEALQKKLEELELDEQQRKRLEAFLTQKQKVGELKDDDFEKISEL
            GAGNGGVVFKVSHKPSGLVMARKLIHLEIKPAIRNQIIRELQVLHECNSPYIVGFYGAFYSDGEISICMEHMDG
            GSLDQVLKKAGRIPEQILGKVSIAVIKGLTYLREKHKIMHRDVKPSNILVNSRGEIKLCDFGVSGQLID{AA00
            37}MAN{AA0037}FVGTRSYMSPERLQGTHYSVQSDIWSMGLSLVEMAVGRYPIPPPDAKELELMFGCQVEGD
            AAETPPRPRTPGRPLSSYGMDSRPPMAIFELLDYIVNEPPPKLPSGVFSLEFQDFVNKCLIKNPAERADLKQLM
            VHAFIKRSDAEEVDFAGWLCSTIGLNQPSTPTHAAGV
         </bpforms:ProteinForm>
      </rdf:Description>
   </rdf:RDF>
</component>
...
```

**Box S4. *BpForms* can help CellML describe the semantic meaning of components which represent macromolecules.** For example, *BpForms* can help CellML describe that the ypp variable in the Wang MAPK cascade model [21] represents a biphosphorylated form of MEK (UniProt: Q0275).

capture several types of missing information about polymers; *BpForms* is both human and machine-readable; *BpForms* is backward compatible with the IUPAC/IUBMB format; and *BpForms* can be integrated into omics, systems biology, and synthetic biology formats such as BioPAX, CellML, SBML, and SBOL.

## Consistency in representing DNA, RNA, and proteins

Like the IUPAC/IUBMB format, *BpForms* can represent DNA, RNA, and proteins. In contrast, the MODOMICS nomenclature only represents RNA and the Biological Expression Language (BEL) [47], PRO, and ProForma only represent proteins.

We anticipate that *BpForms*' consistent representation of DNA, RNA, and proteins will facilitate the adoption of *BpForms*, as well as facilitate the integration of information about epigenetic, post-transcriptional, and post-translational modification into comprehensive maps, models, and genetic designs.

## Capability to concretely represent the chemical structure of polymers

Like molecular formats such as the International Chemical Identifier (InChI) [42], the Protein Data Bank (PDB) format [48] and the Simplified Molecular-Input Line-Entry System (SMILES) [46], *BpForms* can represent the molecular structure of polymers including non-canonical residues,

```
...

<sbol:Sequence>
   <sbol:elements>
      GGGCCUGUAGCUCAGC{8U}GG{8U}{8U}AGAGCGCACGCCUGAU{62A}AGCGUGAG{7G}UCGAUGG{5U}{9U}C
      GAGUCCAUUCAGGCCCACCA
   </sbol:elements>
   <sbol:encoding rdf:resource="http://edamontology.org/format_3909#rna"/>
</sbol:Sequence>

...
```

**Box S5. *BpForms* can help SBOL describe DNA, RNA, and protein parts.** For example, *BpForms* can help SBOL describe the post-transcriptional modifications required for *Bacillus subtilis* $tRNA^{Ile}$ 69 (KEGG: BSU_tRNA_69, SynBioHub: BO_28687).

| | Format | DNA | RNA | Proteins | NC residues, alphabet | NC residues, user defined | Crosslinks | Nicks | Concrete semantics | Capture knowledge gaps | Abstracts structures | User-defined alphabets | Human-readable | Machine-readable | Software tools | Backward compatible | Composable |
|---|---|---|---|---|---|---|---|---|---|---|---|---|---|---|---|---|---|
| Notation | *BpForms* | ✓ | ✓ | ✓ | ✓ | ✓ | ✓ | ✓ | ✓ | ✓ | ✓ | ✓ | ✓ | ✓ | ✓ | ✓ | ✓ |
| | InChI [42] | ✓ | ✓ | ✓ | | × | ✓ | ✓ | ✓ | | | | | ✓ | ✓ | | ✓ |
| | IUPAC/IUBMB [43] | ✓ | ✓ | ✓ | | | | | ✓ | | ✓ | ✓ | | ✓ | ✓ | ✓ | ✓ |
| | MODOMICS nomenclature [44] | | ✓ | | ✓ | | | | × | | ✓ | ✓ | | | | ✓ | ✓ |
| | PRO proteoform format [45] | | | ✓ | ✓ | | × | × | | × | ✓ | | ✓ | × | | | ✓ |
| | ProForma [41] | | | ✓ | ✓ | × | | | | × | ✓ | ✓ | × | | | × | ✓ |
| | SMILES [46] | ✓ | ✓ | ✓ | | × | ✓ | ✓ | ✓ | | | | | ✓ | ✓ | | ✓ |
| Container | BEL [47] | | | ✓ | ✓ | | | | | | ✓ | | ✓ | ✓ | ✓ | | ✓ |
| | BioPAX [13] | ✓ | ✓ | ✓ | × | | ✓ | | | | ✓ | ✓ | | ✓ | ✓ | | |
| | Protein Data Bank (PDB) format [48] | ✓ | ✓ | ✓ | ✓ | × | ✓ | ✓ | ✓ | | ✓ | | | ✓ | ✓ | | |
| | SBOL [22] | ✓ | ✓ | ✓ | | | | | | | ✓ | ✓ | | ✓ | ✓ | | |

**Table S1. Comparison between *BpForms* and other formats for describing polymers.** Each ✓ indicates a feature of a format; each × indicates a partially-supported feature of a format.

crosslinks, and nicks. In contrast, BEL, BioPAX, the MODOMICS nomenclature, the PRO format, ProForma, and SBOL do not represent the bonding of non-canonical residues or nicks, and only BioPAX has limited abilities to represent crosslinks.

We anticipate that the concrete chemical semantics of *BpForms* will help researchers compare and integrate information into comprehensive networks of cellular biochemistry.

### Capability to represent missing information

Similar to the PRO format, *BpForms* can capture several types of missing information about polymers such as the locations non-canonical residues; the structures, masses, and charges of non-canonical residues; and the locations of crosslinks. In contrast, ProForma can only represent missing knowledge about the structures and masses of residues. BEL, BioPAX, InChI, the MODOMICS nomenclature, the PDB format, SBOL, and SMILES cannot represent missing knowledge.

We believe that the ability to represent missing knowledge makes *BpForms* well-suited for omics, WC modeling, and whole-genome engineering which need to represent both knowledge and gaps in knowledge.

### Human readability: abstraction of chemistry

*BpForms* uses alphabets of residues and an ontology of crosslinks to abstract the structures of polymers. These abstractions make *BpForms*-encoded descriptions of polymers easy to read and write. Furthermore, users can define their own abstractions within descriptions of polymers or define their own alphabet of residues or ontology of crosslinks. This enables *BpForms* to represent newly discovered and synthetic residues. BEL, the IUPAC/IUBMB format, the MODOMICS nomenclature,

the PRO format, and ProForma are similarly human-readable.

Although the PDB format uses an alphabet, PDB documents are hard to read and write because the format has limited abilities to abstract residues which do not belong to the alphabet, the format has limited abilities to abstract crosslinks, the format does not abstract nicks, and the format is verbose. Molecular formats such as SMILES are not readable for large molecules such as proteins. BioPAX and SBOL are also difficult to read and write because they are verbose.

**Machine-readability: formal grammar**

Like BEL, BioPAX, InChI, IUPAC/IUBMB, the PDB format, SMILES, and SBOL, *BpForms* is machine-readable because it has a formal grammar. We have used this grammar to build software tools for parsing, validating, calculating properties, exporting, and composing *BpForms*-encoded descriptions of polymers into computational workflows. In contrast, the MODOMICS nomenclature, the PRO format, and ProForma are not machine-readable because we are not aware of formal grammars or software tools for these formats.

**Backward compatibility with IUPAC/IUBMB and sequence informatics tools**

Like the MODOMICS nomenclature and ProForma, *BpForms* maximizes compatibility with sequence informatics tools by generalizing the IUPAC/IUBMB format. As a result, *BpForms* can be integrated into FASTA documents. In contrast, BEL, BioPAX, InChI, the PDB format, the PRO format, SBOL, and SMILES are less compatible with sequence informatics tools because they are not backward compatible with the IUPAC/IUBMB format.

**Composability with other formats**

*BpForms* is compact like other text formats such as BEL, the IUPAC/IUBMB format, the MODOMICS nomenclature, the PRO format, and ProForma. This makes *BpForms* composable with formats for describing entire pathways, models, and genetic design such as BioPAX, CellML, SBML, and SBOL. In contrast, BioPAX, the PDB format, and SBOL are less suited to integration into other formats because they are verbose.

## 11.2. Comparison of *BpForms* alphabets with other alphabet-like resources

Several databases have been developed to help exchange information about non-canonical DNA, RNA, and proteins residues. As described below and summarized in Table S2, we believe that the *BpForms* alphabets are better suited to omics, systems biology, and synthetic biology research because they represent DNA, RNA, and proteins; they represent concrete chemical structures and bonding sites; and they are the most comprehensive collections of residues.

**Consistency in representing DNA, RNA, and proteins**

Like the Protein Data Bank (PDB) Chemical Component Dictionary (CCD) [3], the *BpForms* alphabets represent DNA, RNA, and protein residues. This consistency makes *BpForms* easy to use and facilitates the integration of information, models, and genetic designs that involve DNA, RNA, and proteins. In contrast, DNAmod and REPAIRtoire only represent DNA residues, MODOMICS and the RNA Modification Database only represent RNA residues, and the Protein Modification Ontology (MOD) and RESID only represent protein residues.

**Concreteness of chemical semantics**

Like the PDB CCD, the *BpForms* alphabets define complete residues and each residue defines a concrete chemical structure and concrete bonding sites with the preceding and following residues. This enables *BpForms* to represent the primary structures of non-canonical polymers. This also enables *BpForms* to capture modifications to the sugar-phosphate backbone of DNA and RNA.

| Alphabet | DNA | RNA | Protein | Complete residues | Structures | Bonding | Structure-based | Biochemistry-based |
|---|---|---|---|---|---|---|---|---|
| *BpForms* | 422 | 378 | 1,435 | ✓ | ✓ | ✓ | ✓ | ✓ |
| DNAmod [4] (verified nucleobases) | 58 | | | | ✓ | | | ✓ |
| REPAIRtoire [5] (monophosphates) | 34 | | | ✓ | ✓ | | | ✓ |
| MODOMICS [44] | | 172 | | | ✓ | | | ✓ |
| RNA Modification Database [7] | | 112 | | | ✓ | | | ✓ |
| PDB CCD [3] (unambiguous released residues) | 373 | 271 | 1,095 | ✓ | ✓ | ✓ | ✓ | |
| Protein Modification Ontology (MOD) [49] (leaves) | | | 1,445 | × | × | | × | ✓ |
| RESID [8] | | | 621 | | ✓ | | | ✓ |

**Table S2. Comparison between *BpForms* and other collections of DNA, RNA, and protein residues.** Each ✓ indicates a feature of a collection; each × indicates a partially-supported feature of a collection.

In contrast, DNAmod, MODOMICS, and RNA Modification Database have limited abilities to represent non-canonical DNA and RNA because these formats do represent the sugar-phosphate backbone and the formats have ambiguous chemical semantics because they do not capture bonding sites; REPAIRtoire and RESID have ambiguous chemical semantics because they do not represent bonding sites; and most MOD entries have ambiguous chemical semantics because they do not define concrete structures or bonding sites.

**Breadth of residues from structural and biochemical studies**
To make *BpForms* useful for structural biology, omics, systems biology, and synthetic biology, we populated the *BpForms* alphabets with residues that are important for a wide range of research. As a result, the *BpForms* alphabets are the most comprehensive collections of residues. In contrast, the PDB CCD represents fewer residues because it is primarily based on structural biology data and DNAmod, MOD, MODOMICS, REPAIRtoire, the RNA Modification Database, and RESID represent fewer residues because they are mainly based on biochemical data.

## 11.3. Comparison of the *BpForms* crosslink ontology with other resources

Several resources include information about crosslinks. As illustrated in Table S3, we believe that the *BpForms* crosslink ontology is better suited for omics and systems and synthetic biology research because it concretely represents crosslinks and it is composable with the residues in the *BpForms* alphabets into descriptions of macromolecules. In contrast, REPAIRtoire [5], the Protein Modification Ontology (MOD) [49], and RESID [8] use residues to indirectly represent crosslinks, and the crosslinks in the UniProt controlled vocabulary of posttranslational modifications [17] do not have concrete chemical semantics. As a result, the crosslinks represented by these resources are difficult to compose into macromolecules.

## 11.4. Comparison of *BcForms* grammar with other formats for complexes

Despite the importance of complexes, only a few formats have been developed to represent complexes. As described below and summarized in Table S4, we believe that *BcForms* is better suited

| Resource | Direct representation | Concrete semantics | Composable |
|---|---|---|---|
| *BpForms* | ✓ | ✓ | ✓ |
| Protein Data Bank (PDB) [48] | ✕ | ✓ | |
| Protein Modification Ontology (MOD) [49] | | ✕ | |
| REPAIRtoire [5] | | ✕ | |
| RESID [8] | | ✓ | |
| UniProt [17] | ✓ | | |

**Table S3. Comparison between the *BpForms* crosslinks ontology and other resources that describe crosslinks.** Each ✓ indicates a feature of a resource; each ✕ indicates a partially-supported feature of a resource.

for omics, systems biology, and synthetic biology research because it is the first format that abstractly represents the primary structure of complexes and it is human-readable, machine-readable, and composable with formats for network research such as CellML and SBML.

**Capability to represent the chemical structure of complexes**

Like InChI, the PDB format, and SMILES, *BcForms* can represent the primary structure of complexes, including non-canonical subunits and interchain crosslinks. In contrast, BioPAX and SBOL have limited abilities to represent crosslinks. We anticipate that the concrete semantics of *BcForms* will facilitate the integration of data, models, and genetic designs that involve complexes.

**Abstraction, human readability, and composability**

Similar to BioPAX, and SBOL, *BcForms* abstracts complexes as sets of subunits and crosslinks. This makes *BcForms* human-readable and composable with formats for systems biology and synthetic biology research such as CellML, SBML, and SBOL. By comparison, InChI and SMILES are less human-readable, and the PDB format is both less human-readable and less composable.

## 12. Case studies

Table S5 provides additional information for the synthetic biology case study discussed in the main text.

## 13. Acronyms

**APT** Advanced Package Tool [50]

**BEL** Biological Expression Language [47]

**BNF** Backus-Naur Form

**COMBINE** Computational Modeling in Biology Network [51]

**EBNF** Extended Backus-Naur Form [1]

**InChI** International Chemical Identifier [42]

**MOD** Protein Modification Ontology [49]

| Format | Concrete semantics | Abstracts structures | Human-readable | Machine-readable | Software tools | Composable |
|---|---|---|---|---|---|---|
| *BcForms* | ✓ | ✓ | ✓ | ✓ | ✓ | ✓ |
| BioPAX [13] | | ✓ | | ✓ | ✓ | |
| International Chemical Identifier (InChI) [42] | ✓ | | | ✓ | ✓ | ✓ |
| Protein Data Bank (PDB) format [48] | ✓ | ✕ | | ✓ | ✓ | |
| Synthetic Biology Open Language (SBOL) [22] | | ✓ | | ✓ | ✓ | |
| Simplified Molecular-Input Line-Entry System (SMILES) [46] | ✓ | | | ✓ | ✓ | ✓ |

**Table S4. Comparison between *BcForms* and other formats for describing complexes.** Each ✓ indicates a feature of a format; each ✕ indicates a partially-supported feature of a format.

| PDB CCD id | RESID id | Name | PDB entries | Proteins | Absence from *E. coli* |
|---|---|---|---|---|---|
| HYP | AA0030 | 4-hydroxyproline | 239 | Collagen and plant walls | [52–54] |
| HIC | AA0317 | 4-methyl-histidine | 121 | Actin and myosin | [55, 56] |
| MEN | AA0070 | N-methyl asparagine | 57 | Antennae of photosystem II | [57–59] |
| FVA | | N-formyl-L-valine | 23 | Gramicidin | |
| 6V1 | | | 10 | | |
| TQQ | | | 8 | Aromatic amine dehydrogenase | |
| TRX | | 6-hydroxytryptophan | 6 | RNA polymerase II | |
| PSW | | 3-(sulfanylselanyl)-L-alanine | 5 | | |

**Table S5.** The most common protein residues within the Protein Data Bank (PDB) which cannot be synthesized by *Escherichia coli*. We identified these residues by using *BpForms* to analyze the PDB, and we confirmed the absence of the most frequent residues from *E. coli* via the literature. This information could be used to constrain the design of novel strains of *E. coli*. For example, genetic designs based on *E. coli* should not include photosystem II, or such designs should also include phycobiliprotein asparagine methyltransferase CpcM [58].

**PDB** Protein Data Bank [48]

**PDB CCD** PDB Chemical Component Dictionary [3]

**PRO** Protein Ontology [45]

**REST** Representational State Transfer

**SBML** Systems Biology Markup Language [16]

**SBOL** Synthetic Biology Open Language [22]

**SMILES** Simplified Molecular-Input Line-Entry System [46]

**SVG** Scalable Vector Graphics [30]

**WC** Whole-cell [18, 19]

# References

1. Wikipedia. *Extended Backus-Naur Form.* https://en.wikipedia.org/wiki/Extended_Backus-Naur_form (2019).

2. Shinan, E. *Lark – a modern parsing library for Python.* https://lark-parser.readthedocs.io.

3. Westbrook, J. D., Shao, C., Feng, Z., Zhuravleva, M., Velankar, S. & Young, J. The Chemical Component Dictionary: complete descriptions of constituent molecules in experimentally determined 3D macromolecules in the Protein Data Bank. *Bioinformatics* **31,** 1274–1278 (2014).

4. Sood, A. J., Viner, C. & Hoffman, M. M. DNAmod: the DNA modification database. *J. Cheminform.* **11,** 30 (2019).

5. Milanowska, K., Krwawicz, J., Papaj, G., Kosiński, J., Poleszak, K., Lesiak, J., Osińska, E., Rother, K. & Bujnicki, J. M. REPAIRtoire–a database of DNA repair pathways. *Nucleic Acids Res.* **39,** D788–D792 (2010).

6. Machnicka, M. A., Milanowska, K., Osman Oglou, O., Purta, E., Kurkowska, M., Olchowik, A., Januszewski, W., Kalinowski, S., Dunin-Horkawicz, S., Rother, K. M., *et al.* MODOMICS: a database of RNA modification pathways–2013 update. *Nucleic Acids Res.* **41,** D262–D267 (2012).

7. Cantara, W. A., Crain, P. F., Rozenski, J., McCloskey, J. A., Harris, K. A., Zhang, X., Vendeix, F. A., Fabris, D. & Agris, P. F. The RNA Modification Database, RNAMDB: 2011 update. *Nucleic Acids Res.* **39,** D195–D201 (2010).

8. Garavelli, J. S. The RESID Database of Protein Modifications as a resource and annotation tool. *Proteomics* **4,** 1527–1533 (2004).

9. ChemAxon Limited. *Marvin.* https://chemaxon.com/products/marvin (2019).

10. O'Boyle, N. M., Guha, R., Willighagen, E. L., Adams, S. E., Alvarsson, J., Bradley, J.-C., Filippov, I. V., Hanson, R. M., Hanwell, M. D., Hutchison, G. R., *et al.* Open data, open source and open standards in chemistry: the Blue Obelisk five years on. *J. Cheminform.* **3,** 37 (2011).

11. Pearson, W. R. Rapid and sensitive sequence comparison with FASTP and FASTA. *Methods Enzymol.* **183,** 63–98 (1990).

12. Cock, P. J., Antao, T., Chang, J. T., Chapman, B. A., Cox, C. J., Dalke, A., Friedberg, I., Hamelryck, T., Kauff, F., Wilczynski, B., *et al.* Biopython: freely available Python tools for computational molecular biology and bioinformatics. *Bioinformatics* **25,** 1422–1423 (2009).

13. Demir, E., Cary, M. P., Paley, S., Fukuda, K., Lemer, C., Vastrik, I., Wu, G., D'eustachio, P., Schaefer, C., Luciano, J., *et al.* The BioPAX community standard for pathway data sharing. *Nat. Biotechnol.* **28,** 935 (2010).

14. Bergmann, F. T., Rodriguez, N. & Le Novère, N. COMBINE archive specification version 1. *J. Integr. Bioinform.* **12,** 104–118 (2015).

15. Cuellar, A., Hedley, W., Nelson, M., Lloyd, C., Halstead, M., Bullivant, D., Nickerson, D., Hunter, P. & Nielsen, P. The CellML 1.1 specification. *J. Integr. Bioinform.* **12,** 4–85 (2015).

16. Hucka, M., Bergmann, F. T., Dräger, A., Hoops, S., Keating, S. M., Le Novère, N., Myers, C. J., Olivier, B. G., Sahle, S., Schaff, J. C., *et al.* The Systems Biology Markup Language (SBML): language specification for level 3 version 2 core. *J. Integr. Bioinform.* **15** (2018).

17. UniProt Consortium *et al.* UniProt: the universal protein knowledgebase. *Nucleic Acids Res.* **46,** 2699 (2018).

18. Karr, J. R., Sanghvi, J. C., Macklin, D. N., Gutschow, M. V., Jacobs, J. M., Bolival Jr, B., Assad-Garcia, N., Glass, J. I. & Covert, M. W. A whole-cell computational model predicts phenotype from genotype. *Cell* **150,** 389–401 (2012).

19. Goldberg, A. P., Szigeti, B., Chew, Y. H., Sekar, J. A., Roth, Y. D. & Karr, J. R. Emerging whole-cell modeling principles and methods. *Curr. Opin. Biotechnol.* **51,** 97–102 (2018).

20. Tyson, J. J. Modeling the cell division cycle: cdc2 and cyclin interactions. *Proc. Natl. Acad. Sci. U. S. A.* **88,** 7328–7332 (1991).

21. Wang, C.-C., Cirit, M. & Haugh, J. M. PI3K-dependent cross-talk interactions converge with Ras as quantifiable inputs integrated by Erk. *Mol. Syst. Biol.* **5** (2009).

22. Cox, R. S., Madsen, C., McLaughlin, J. A., Nguyen, T., Roehner, N., Bartley, B., Beal, J., Bissell, M., Choi, K., Clancy, K., *et al.* Synthetic Biology Open Language (SBOL) version 2.2.0. *J. Integr. Bioinform.* **15** (2018).

23. Karr, J. R. *SBOL SEP 033 – Concrete descriptions of non-canonical DNA, RNA, and proteins.* https://github.com/SynBioDex/SEPs/blob/master/sep_033.md.

24. Python Software Foundation. *Python.* https://python.org/ (2019).

25. Richardson, L. *Beautiful Soup.* https://www.crummy.com/software/BeautifulSoup/ (2019).

26. Reitz, K., Cordasco, I. & Prewit, N. *Requests: HTTP for humans.* https://2.python-requests.org (2019).

27. Bayer, M. *SQLAlchemy – The database toolkit for Python.* https://www.sqlalchemy.org/ (2019).

28. Ben-Kiki, O., Evans, C. & döt Net, I. *YAML: YAML Ain't Markup Language.* https://yaml.org (2019).

29. Van der Neut, A. *ruamel.yaml.* https://yaml.readthedocs.io (2019).

30. W3C SVG Working Group. *Scalable Vector Graphics (SVG).* https://www.w3.org/Graphics/SVG/ (2019).

31. Data Folk Labs. *Cement framework.* https://builtoncement.com/ (2019).

32. Haustant, A. *Flask-RESTPlus.* https://flask-restplus.readthedocs.io (2019).

33. ZURB, Inc. *Foundation – The most advanced responsive front-end framework in the world.* https://foundation.zurb.com (2019).

34. Skarnelis, J. *FancyBox – Fancy jQuery lightbox alternative.* http://fancybox.net (2019).

35. Phusion Holding B.V. *Passenger.* https://www.phusionpassenger.com (2019).

36. Python Software Foundation. *unittest unit testing framework.* https://docs.python.org/3/library/unittest.html (2019).

37. Batchelder, N. *Coverage.py.* https://coverage.readthedocs.io (2019).

38. Goodger, D. *reStructuredText.* http://docutils.sourceforge.net/rst.html (2019).

39. Brandl, G. *et al. Sphinx – Python documentation generator.* http://www.sphinx-doc.org (2019).

40. Project Jupyter. *Jupyter.* https://jupyter.org (2019).

41. LeDuc, R. D., Schwämmle, V., Shortreed, M. R., Cesnik, A. J., Solntsev, S. K., Shaw, J. B., Martin, M. J., Vizcaino, J. A., Alpi, E., Danis, P., *et al.* ProForma: a standard proteoform notation. *J. Proteome Res.* **17,** 1321–1325 (2018).

42. Heller, S. R., McNaught, A., Pletnev, I., Stein, S. & Tchekhovskoi, D. InChI, the IUPAC international chemical identifier. *J. Cheminform.* **7,** 23 (2015).

43. Leonard, S. A. IUPAC/IUB single-letter codes within nucleic acid and amino acid sequences. *Curr. Protoc. Bioinformatics,* A–1A (2003).

44. Boccaletto, P., Machnicka, M. A., Purta, E., Piątkowski, P., Bagiński, B., Wirecki, T. K., de Crécy-Lagard, V., Ross, R., Limbach, P. A., Kotter, A., *et al.* MODOMICS: a database of RNA modification pathways. 2017 update. *Nucleic Acids Res.* **46,** D303–D307 (2017).

45. Natale, D. A., Arighi, C. N., Blake, J. A., Bona, J., Chen, C., Chen, S.-C., Christie, K. R., Cowart, J., D'Eustachio, P., Diehl, A. D., *et al.* Protein Ontology (PRO): enhancing and scaling up the representation of protein entities. *Nucleic Acids Res.* **45,** D339–D346 (2016).

46. Weininger, D. SMILES, a chemical language and information system. 1. Introduction to methodology and encoding rules. *J. Chem. Inform. Comp. Sci.* **28,** 31–36 (1988).

47. Fluck, J., Madan, S., Ansari, S., Karki, R., Rastegar-Mojarad, M., Catlett, N. L., Hayes, W., Szostak, J., Hoeng, J., Peitsch, M., *et al.* Training and evaluation corpora for the extraction of causal relationships encoded in biological expression language (BEL). *Database* **2016** (2016).

48. Westbrook, J. D. & Fitzgerald, P. in *Structural Bioinformatics* (eds Bourne, P. E. & Weissig, H.) 161–179 (Wiley Online Library, 2003).

49. Montecchi-Palazzi, L., Beavis, R., Binz, P.-A., Chalkley, R. J., Cottrell, J., Creasy, D., Shofstahl, J., Seymour, S. L. & Garavelli, J. S. The PSI-MOD community standard for representation of protein modification data. *Nat. Biotechnol.* **26,** 864 (2008).

50. Ubuntu Documentation Team. *Apt* https://help.ubuntu.com/lts/serverguide/apt.html.

51. Hucka, M., Nickerson, D. P., Bader, G. D., Bergmann, F. T., Cooper, J., Demir, E., Garny, A., Golebiewski, M., Myers, C. J., Schreiber, F., *et al.* Promoting coordinated development of community-based information standards for modeling in biology: the COMBINE initiative. *Front. Bioeng. Biotechnol.* **3,** 19 (2015).

52. Pinkas, D. M., Ding, S., Raines, R. T. & Barron, A. E. Tunable, post-translational hydroxylation of collagen domains in Escherichia coli. *ACS Chem. Biol.* **6,** 320–324 (2011).

53. An, B., Kaplan, D. L. & Brodsky, B. Engineered recombinant bacterial collagen as an alternative collagen-based biomaterial for tissue engineering. *Front. Chem.* **2,** 40 (2014).

54. Yi, Y., Sheng, H., Li, Z. & Ye, Q. Biosynthesis of trans-4-hydroxyproline by recombinant strains of Corynebacterium glutamicum and Escherichia coli. *BMC Biotechnol.* **14,** 44 (2014).

55. Kwiatkowski, S., Seliga, A. K., Vertommen, D., Terreri, M., Ishikawa, T., Grabowska, I., Tiebe, M., Teleman, A. A., Jagielski, A. K., Veiga-da Cunha, M., *et al.* SETD3 protein is the actin-specific histidine N-methyltransferase. *Elife* **7,** e37921 (2018).

56. Xiao, H., Peters, F. B., Yang, P.-Y., Reed, S., Chittuluru, J. R. & Schultz, P. G. Genetic incorporation of histidine derivatives using an engineered pyrrolysyl-tRNA synthetase. *ACS Chem. Biol.* **9,** 1092–1096 (2014).

57. Klotz, A. & Glazer, A. N. gamma-N-methylasparagine in phycobiliproteins. Occurrence, location, and biosynthesis. *J. Biol. Chem.* **262,** 17350–17355 (1987).

58. Shen, G., Leonard, H. S., Schluchter, W. M. & Bryant, D. A. CpcM posttranslationally methylates asparagine-71/72 of phycobiliprotein beta subunits in Synechococcus sp. strain PCC 7002 and Synechocystis sp. strain PCC 6803. *J. Bacteriol.* **190,** 4808–4817 (2008).

59. Scheer, H & Zhao, K.-H. Biliprotein maturation: the chromophore attachment. *Mol. Microbiol.* **68,** 263–276 (2008).
